# Supplementary material for: Multilevel nested simulation for efficient risk estimation
Source: arXiv:1802.05016 ancillary file (2019-02-14)
Supplement: Supplementary file 1 [file model-problem.pdf]

# SUPPLEMENTARY MATERIALS: MULTILEVEL NESTED SIMULATION FOR EFFICIENT RISK ESTIMATION *

MICHAEL B. GILES † AND ABDUL-LATEEF HAJI-ALI†

**Abstract.** In this document, we explain in more details the model problem that was presented in the main work. We also repeat some of the discussion from the main manuscript to make the current document self-contained.

The model problem that we consider is a simple example that mimics many of the challenges of computing the probability of a large loss from a financial portfolio. Assuming we have a stock, $W$, following a Brownian Motion and a final payoff function, $f(x) = -x^2$ evaluated at maturity, $T = 1$, the value function for the option is

$$V(t,x) = \mathbb{E}[f(W(1)) \mid W(t) = x] = \mathbb{E}\left[-\left(x + (1-t)^{1/2} Z\right)^2\right]$$

for $t \in [0,1]$ and $Z$ being a standard normal variable. Note that the portfolio consisting of this one option is Delta-neutral, $\frac{\partial V}{\partial x}(0,0) = 0$, and has negative Gamma, $\frac{\partial V^2}{\partial x^2} = -2$. Hence a large loss is incurred with very low probability under extreme circumstances. Here, the loss is defined as the difference between future, at some risk horizon $\tau \ll 1$, and current risk-neutral portfolio expectations. That is, the loss is $V(0,0) - V(\tau, x)$ given that the stock value at $\tau$ is $x$.

We are interested in the probability, $\eta$, of the portfolio loss exceeding a given loss level, $L_\eta$, i.e.,

$$\eta = \mathbb{E}\left[\mathrm{H}\left(V(0,0) - V(\tau, W(\tau)) - L_\eta\right)\right]. \tag{SM0.1}$$

Alternatively, one may specify $\eta \ll 1$ and determine the corresponding loss level, $L_\eta$, using the relation (SM0.1). Defining

$$\begin{aligned} P(y,z) &:= -\left(\tau^{1/2}\, y + (1-\tau)^{1/2}\, z\right)^2 \\ &= -\tau y^2 - 2\tau^{1/2}(1-\tau)^{1/2} yz - (1-\tau) z^2, \end{aligned}$$

we have that

$$\eta = \mathbb{E}\left[\mathrm{H}\left(\mathbb{E}\left[P(\widetilde{Y}, Z)\right] - \mathbb{E}[P(Y,Z) \mid Y] - L_\eta\right)\right].$$

Note that only the second inner expectation in (SM0.1) is conditioned on samples of the outer random variable, $Y$.

To estimate $\eta = \mathbb{E}[\mathrm{H}(\mathbb{E}[X \mid Y])]$ for some $X$, we have to estimate the two inner expectations, $\mathbb{E}[P(\widetilde{Y}, Z)]$ and $\mathbb{E}[P(Y,Z) \mid Y]$ for a given $Y$. We could use the exact value of $\mathbb{E}[P(\widetilde{Y}, Z)] = -1$ and set $X := -1 - P(Y,Z) - L_\eta$. However, the variance is $\mathrm{Var}[X|Y] = 4\tau(1-\tau)Y^2 + 2(1-\tau)^2 = \mathcal{O}(1)$. We could also use independent samples of $Z$ to compute both $\mathbb{E}\left[P(\widetilde{Y}, Z)\right]$ and $\mathbb{E}[P(Y,Z) \mid Y]$, setting $X := P(\widetilde{Y}, \widetilde{Z}) - P(Y,Z) - L_\eta$ for independent standard normal variables $Z$, $\widetilde{Z}$ and $\widetilde{Y}$. The variance would then be $\mathrm{Var}[X \mid Y] = 2(1-\tau)^2 + 4\tau(1-\tau)Y^2 + 2 = \mathcal{O}(1)$.

---

*Submitted 28 February 2018.

†University of Oxford (mike.giles@maths.ox.ac.uk, hajiali@maths.ox.ac.uk).

Instead, we use the same samples of $Z$ when estimating both inner expectations. Moreover, for increased variance reduction, we also use an antithetic control variate based on the fact that $\widetilde{Y}$ is identically distributed to $-\widetilde{Y}$. In summary, we set, for a given $Y$,

$$\begin{aligned} X &\coloneqq \frac{1}{2}\Big(P(\widetilde{Y}, Z) + P(-\widetilde{Y}, Z)\Big) - P(Y, Z) - L_\eta \\ &= \tau(Y^2 - \widetilde{Y}^2) + 2\tau^{1/2}(1-\tau)^{1/2}\, YZ - L_\eta. \end{aligned} \tag{SM0.2}$$

Here, again, $\widetilde{Y}$ and $Z$ are independent standard normal random variables. The variance in this case is reduced to

$$\sigma^2 = \mathrm{Var}[X \mid Y] = 2\tau^2 + 4\tau(1-\tau)Y^2 = \mathcal{O}(\tau).$$

and we can also compute analytically

$$d = |\mathbb{E}[X \mid Y]| = \big|\tau\big(Y^2 - 1\big) - L_\eta\big| = \big|\tau\big(Y^2 - Y_\eta^2\big)\big|.$$

where $Y_\eta^2 = 1 + L_\eta/\tau$. Moreover, the cumulative distribution function (CDF) of the random variable, $\mathbb{E}[X \mid Y]$, is

$$\begin{aligned} \mathbb{P}[\mathbb{E}[X \mid Y] \le x] &= \mathbb{P}\Big[\mathbb{E}\Big[P(\widetilde{Y}, Z)\Big] - \mathbb{E}[P(Y,Z) \mid Y] - L_\eta \le x\Big] \\ &= \mathbb{P}\left[|Y| \le \left(\frac{\tau + x + L_\eta}{\tau}\right)^{1/2}\right] \\ &= 1 - 2\,\Phi\left(-\left(1 + \frac{x + L_\eta}{\tau}\right)^{1/2}\right), \end{aligned} \tag{SM0.3}$$

where $\Phi$ is the standard normal CDF and where we substituted $\mathbb{E}[P(\widetilde{Y}, Z)] = -1$ and $\mathbb{E}[P(Y,Z) \mid Y] = -\tau Y^2 - (1-\tau)$. In particular,

$$\eta = \mathbb{P}[\mathbb{E}[X \mid Y] \ge 0] = 2\,\Phi\left(-\left(1 + \frac{L_\eta}{\tau}\right)^{1/2}\right).$$

We define the signed quantity $\overline{\delta} = \mathbb{E}[X \mid Y]/\sigma$. We also define the positive quantity $\delta = d/\sigma = |\overline{\delta}|$. Below, we will abuse the notation and use $d, \sigma, \delta$ and $\overline{\delta}$ to denote random variables or functions depending on context. That is, we will write $d(Y), \sigma(Y)$, $\overline{\delta}(Y)$ and $\delta(Y)$ to denote corresponding functions of $Y$.

Setting $\tau = 0.02$ and $L_\eta \approx 0.0805$ so that $\eta = 0.025$, Figure SM1 shows the cumulative distribution function of $\mathbb{E}[X|Y]$ and illustrates the square-root behaviour in the neighbourhood of $-\tau - L_\eta$. This figure was obtained by plotting $\mathbb{E}[X \mid Y] = \tau(Y^2 - 1) - L_\eta$ versus $\Phi(Y)$ for a range of values of $Y$. Figure SM2-(a) shows $\mathbb{E}[X \mid Y]$, $\sigma$ and $\overline{\delta}$ versus positive values of $Y$. Note that these quantities are even with respect to $Y$ and monotonically increasing with respect to positive values of $Y$. On the other hand, Figure SM2-(b) plots the CDF of $\overline{\delta}$. This is obtained by computing $\overline{\delta}$ for a range of positive values of $Y$ and plotting it against $1 - 2\Phi(Y)$.

To plot the probability density function (PDF) of $\overline{\delta}$, denoted below by $p$, we have to compute the derivative of its CDF. Given the CDF, this can be done using a simple finite difference approximation. Another way is to compute $\overline{\delta}$ and its PDF as

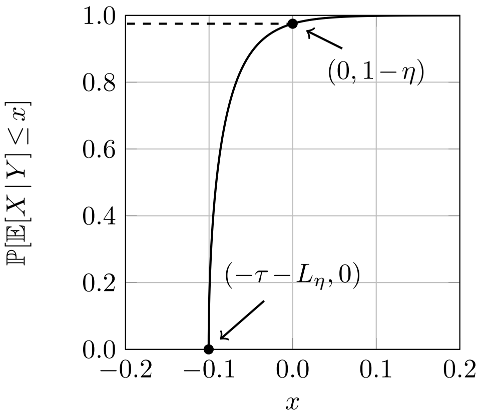


(a)

Fig. SM1: The cumulative distribution function of $\mathbb{E}[X \mid Y]$ with $X$ as defined in (SM0.2) and $Y$ a standard normal variable. This figure illustrates the square-root behaviour in the neighbourhood of $x = -\tau - L_\eta$. Here, we use $\tau = 0.02$ and $L_\eta \approx 0.0805$ so that $\eta = 0.025$.

a function of positive $y$ and plot them against each other. Since $\overline{\delta}$ is a monotonically increasing function of $y$, the PDF of $\overline{\delta}$ is

$$p(\overline{\delta}(y)) = 2\phi(y)\left(\frac{\partial\overline{\delta}(y)}{\partial y}\right)^{-1}, \tag{SM0.4}$$

as a function of $y$, where

$$\frac{\partial\overline{\delta}(y)}{\partial y} = \frac{2\tau\, y}{\sigma} - \frac{4\overline{\delta}\; y\; \tau(1-\tau)}{\sigma^2}$$

and $\phi(y) = \Phi'(y)$ is the standard normal PDF. The factor of 2 in (SM0.4) is because $\overline{\delta}(y) = \overline{\delta}(-y)$. A third way is to write $y^2$ as a function of $\overline{\delta}^2$. This is done by solving the equation $\overline{\delta}^2 = d^2(y)/\sigma^2(y)$ for $y^2$ to find the two real roots

$$y_1^2(\overline{\delta}) = Y_\eta^2 + 2\overline{\delta}^2\left(\frac{1-\tau}{\tau} - \sqrt{\left(\frac{1-\tau}{\tau}\right)^2 + \frac{1}{2\overline{\delta}^2} + \frac{Y_\eta^2}{\overline{\delta}^2}\cdot\frac{1-\tau}{\tau}}\right)$$

$$y_2^2(\overline{\delta}) = Y_\eta^2 + 2\overline{\delta}^2\left(\frac{1-\tau}{\tau} + \sqrt{\left(\frac{1-\tau}{\tau}\right)^2 + \frac{1}{2\overline{\delta}^2} + \frac{Y_\eta^2}{\overline{\delta}^2}\cdot\frac{1-\tau}{\tau}}\right)$$

where $Y_\eta^2 = 1 + L_\eta/\tau$. Note that $\overline{\delta}(y_1) \leq 0$ while $\overline{\delta}(y_2) \geq 0$. Then, the PDF of $\overline{\delta}$, as a function of $\overline{\delta}$, is

$$p(\overline{\delta}) = 2\phi(y_1(\overline{\delta}))\left(\frac{\partial\overline{\delta}(y_1(\overline{\delta}))}{\partial y}\right)^{-1}\mathbf{1}_{\overline{\delta}<0} + 2\phi(y_2(\overline{\delta}))\left(\frac{\partial\overline{\delta}(y_2(\overline{\delta}))}{\partial y}\right)^{-1}\mathbf{1}_{\overline{\delta}\geq 0},$$

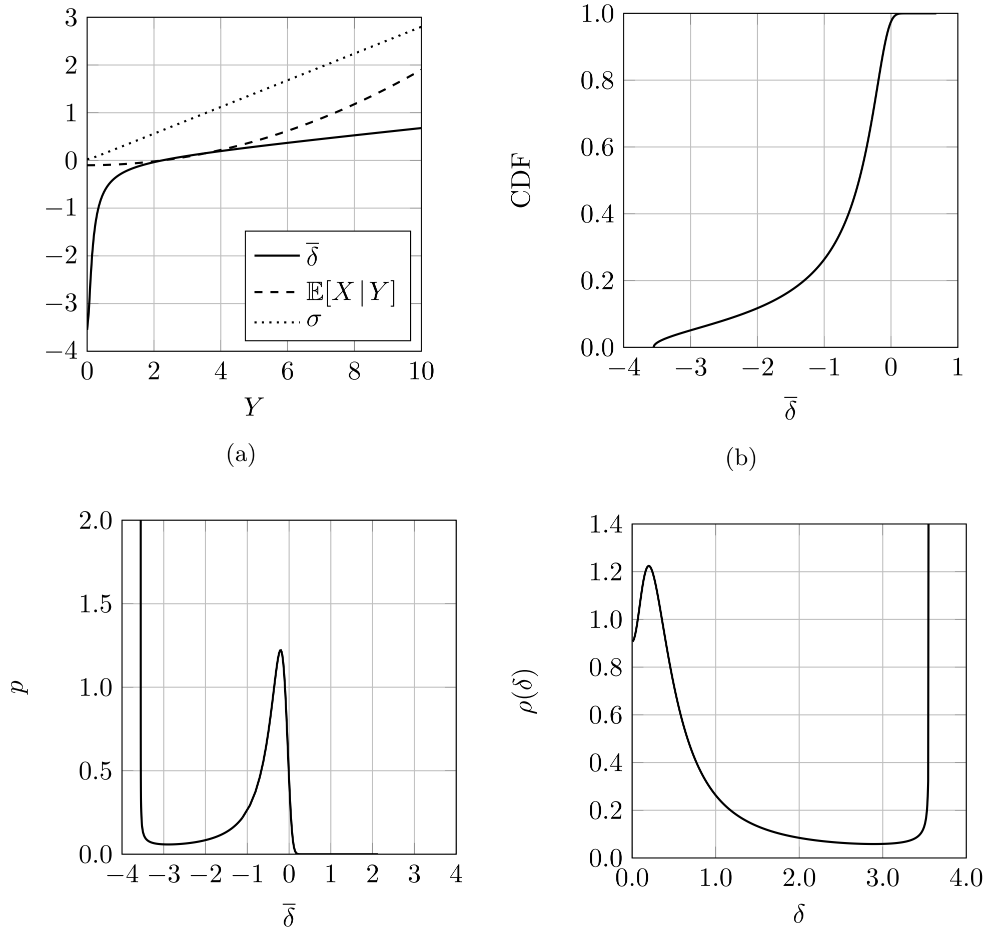


(a) (b) (c) (d)

Fig. SM2: (a) shows that $\overline{\delta}$, $\mathbb{E}[X\,|\,Y]$ and $\sigma$ are monotonically increasing with respect to $Y$, for positive $Y$. (b) and (c) show the CDF and PDF, respectively, of $\overline{\delta}$ while (d) shows the PDF of $\delta$. Both (c) and (d) have an inverse square-root singularity, caused by the square root behaviour in the CDF of $\mathbb{E}[X\,|\,Y]$, cf. (SM0.3). For all figures, we use $\tau = 0.02$ and $L_\eta \approx 0.0805$ so that $\eta = 0.025$.

for any $\overline{\delta}$. Figure SM2-(c) plots the PDF of $\delta$ as obtained by any of the previous three methods. Finally, Figure SM2-(d) shows the PDF of $\delta$. This is obtained by

$$\rho(\delta) = p(\delta) + p(-\delta).$$
